# Supplementary material for: Electronic Structure Evolution during the Growth of Graphene Nanoribbons on Au(110)
Source: arXiv:1704.06373 ancillary file (2017-04-21)
Supplement: Supplementary file 1 [file SI.pdf]

# Supporting information for: Electronic Structure Evolution during the Growth of Graphene Nanoribbons on Au(110)

Ada Della Pia,[*,†] Giulia Avvisati,[†] Oualid Ourdjini,[†] Claudia Cardoso,[‡] Daniele Varsano,[‡] Deborah Prezzi,[‡] Andrea Ferretti,[*,‡] Carlo Mariani,[†] and Maria Grazia Betti[*,†]

†*Department of Physics, La "Sapienza" University, 00185 Roma, Italy*

‡*Centro S3, CNR-Istituto Nanoscienze, 41125 Modena, Italy*

E-mail: Ada.Della.Pia@roma1.infn.it; andrea.ferretti@nano.cnr.it; maria.grazia.betti@roma1.infn.it

# DBBA molecular states

The DBBA molecular states have been determined on a thin-film (about 10 monolayers) deposited at RT on a Au(110) surface, by means of UPS as reported in Fig. S1. Photoemission data have been integrated on a 12°-wide angular window along the direction which forms an angle of 20° with the [001] direction. A background curve (spline curve and Fermi edge) has been subtracted from the spectrum before performing the fitting analysis. The energy of the main peaks are reported in table S1 and have been identified by Gaussian fits, as shown in Fig. S1.

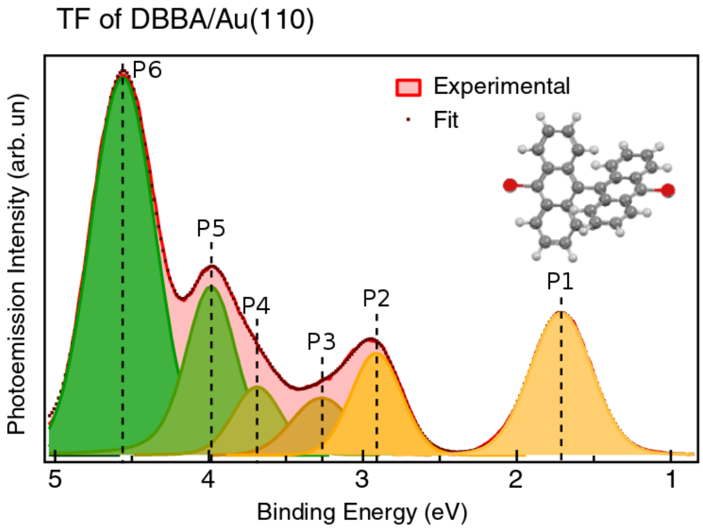


Figure S1: Photoemission spectrum acquired with He-I radiation (red line), whole fitting curve (dotted line) and Gaussian fits of each molecular peak (greenish to orange colored peaks). The peak maxima have been highlighted with vertical lines.

**Table S1: Position of the DBBA electronic states measured with respect to the Fermi level (Binding Energy, ±0.10 eV) and to the vacuum level (Ionization energy), the latter obtained by summing the work function value (4.87 eV) measured for the thin film.**

| Peak | Binding Energy (eV) | Ionization Energy (eV) |
|---|---|---|
| P1 | 1.70 | 6.57 |
| P2 | 2.90 | 7.77 |
| P3 | 3.25 | 8.12 |
| P4 | 3.70 | 8.57 |
| P5 | 4.00 | 8.87 |
| P6 | 4.55 | 9.42 |

# Basis set dependence

In Tab. S2 we report tests about the dependence of the electronic structure of DBBA on the localized basis set used in the calculations. We also report and compare with results obtained using plane-waves and pseudopotentials. According to this data, the use of an augmented basis set is found critical to compare with plane-waves, with an overall agreement on the eigenvalues better than 0.05 eV.

**Table S2: HOMO (top lines) and LUMO (bottom lines) values computed against different localized basis set and plane waves for LDA, PBE, and PBE0 functionals. All values are in eV.**

| | **cc-pVDZ** | **cc-pVTZ** | **aug-cc-pVDZ** | **aug-cc-pVTZ** | **plane waves** |
|---|---|---|---|---|---|
| **LDA** | -5.13 | -5.28 | -5.31 | -5.32 | -5.30 |
| | -2.99 | -3.16 | -3.19 | -3.21 | -3.18 |
| **PBE** | -4.93 | -5.05 | -5.10 | -5.10 | -5.14 |
| | -2.77 | -2.90 | -2.96 | -2.97 | -3.00 |
| **PBE0** | -5.74 | -5.82 | -5.85 | -5.88 | -5.90 |
| | -2.13 | -2.23 | -2.27 | -2.32 | -2.31 |

## Length dependence of the DOS of oligo-anthryl chains

Here we report a study of the dependence of the electronic structure (DOS in particular) of oligo-anthryl molecules on the number of units in the chains. This analysis is relevant in the present context since, experimentally, the polyanthryl units are of finite length. Our results, obtained by using both local and semilocal as well as hybrid functionals (CAM-B3LYP is reported here) do not show any length dependence of the oligo-anthryl DOS (HOMO and LUMO in particular). Calculations have been performed using ORCA (within the cc-pVTZ basis) and Quantum ESPRESSO (plane waves).

**Table S3: HOMO (top lines) and LUMO (bottom lines) values of several oligo-anthryl chains with 1 to 5 bianthracene (BA) units computed at the DFT level using LDA (VWN-5) and CAM-B3LYP functionals. Calculations performed with ORCA used a cc-pVTZ basis. LDA calculations performed with Quantum ESPRESSO (QE) are reported for comparison.**

| | **N=1** | **N=2** | **N=3** | **N=4** | **N=5** |
|---|---|---|---|---|---|
| **LDA** | -5.13 | -5.09 | -5.09 | -5.10 | -5.10 |
| (plane-waves QE) | -2.90 | -2.95 | -2.97 | -2.99 | -3.00 |
| **LDA** | -5.11 | -5.08 | -5.07 | -5.08 | -5.09 |
| (cc-pVTZ ORCA) | -2.88 | -2.93 | -2.95 | -2.96 | -2.98 |
| **CAM-B3LYP** | -6.61 | -6.55 | -6.54 | -6.54 | -6.54 |
| (cc-pVTZ ORCA) | -0.93 | -1.00 | -1.02 | -1.03 | -1.04 |

# Band structure of polyanthryl and GNR

In Fig. S2 we present the band structure of free standing polyanthryl and GNR computed within DFT/LDA as a reference to the band structures of these systems adsorbed on Au(110) shown in Figs. 5 and 6 of the paper. The PA bands are poorly dispersive, as already suggested by the DOS shown in Fig. 5 of the paper.

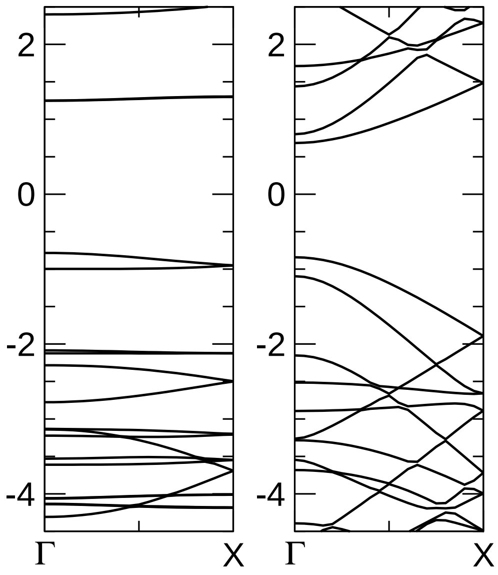


Figure S2: Band structure of free standing polyanthryl and GNR computed within DFT/LDA.

# DBBA on Au(110)

In Fig. S3 we present the density of states of BA adsorbed on Au(110) computed at the LDA level by using Quantum ESPRESSO and projected on the different C atoms. The orange lines correspond to the central C atoms connecting the two lobes of the molecule while the blue lines correspond to the C atoms previously (before dehalogenation) bonded to Br. This result supports the idea that the splitting of the oligo-anthryl peak at -1.0 eV is mainly due to the formation of C-Au bonds.

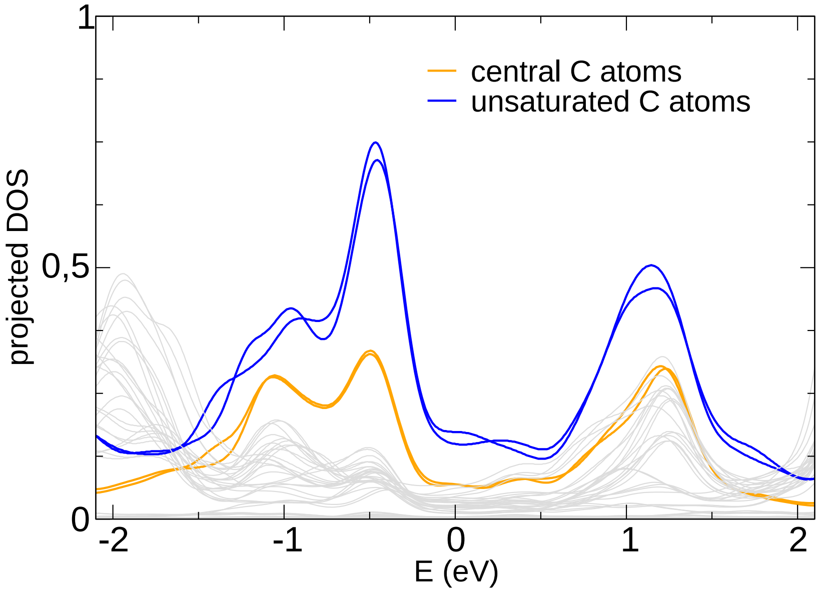


Figure S3: DOS computed for BA on Au(110), projected on the different carbon atoms.

# GNRs on Au(110)

We present here the UPS spectra for DBBA molecules deposited on Au(110) kept at 470 K at increasing coverages, and the corresponding STM images (Fig. S4). At low molecular density, DBBA molecules deposited on Au(110) at 470 K dehalogenate and cyclo-dehydrogenate before any polymerization (bisanthene), adsorbing flat and bridging across the Au rows. At higher coverage, the Au surface reconstructs with a 1×3 periodicity, enlarging the distance between the Au rows and favouring the coalescence of bisanthene units into the channels. The scanning tunneling microscopy image in the inset of Fig. S4 reveals short bisanthene chains aligned along the $[1\bar{1}0]$ direction. A further reconstruction of the Au surface, 1×4, occurs at the completion of a single layer when short C nanostructures appear inside the Au channels. The continuous and diffuse charge density of these structures is compatible with the formation of GNRs, see inset in Fig. S4 and Ref.[S1] The reconstruction of the Au channels determines the final configuration of the GNRs strands, few nm long, while the low molecular diffusion and the adsorption energy hinder the formation of high-density GNRs. Recently, it has been demonstrated that the decrease of molecular surface mobility on the open and anisotropic Cu(110) surface leads only to the formation of bisanthene units, called

nanographene in Ref.[S2] The stronger interaction with the Cu surface completely hinders the covalent coupling of the molecular units and the formation of GNRs.

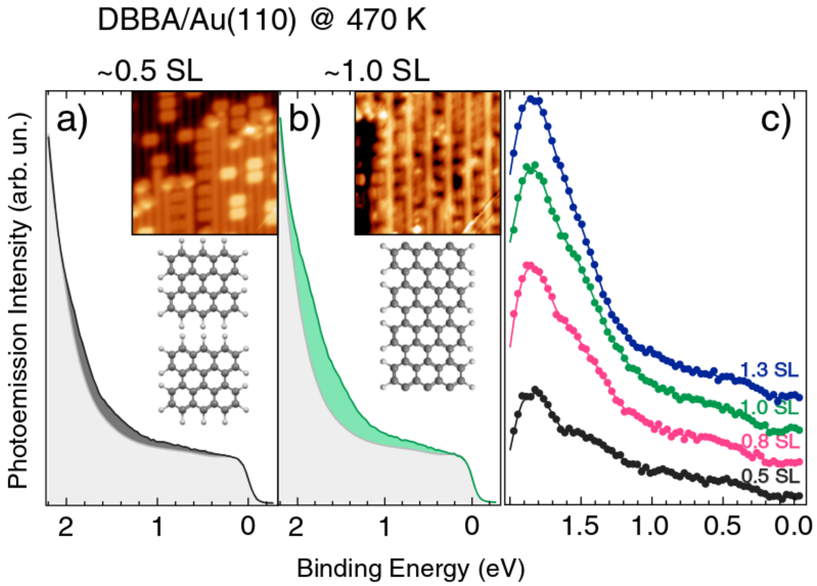


Figure S4: Normal emission UPS spectra for DBBA molecules deposited on Au(110) kept at 470 K at increasing coverages. Scanning tunneling microscopy images[S1] (dimensions: 13.5×13.5 $nm^2$) and sketches of the molecular systems are reported as insets in (a) and (b). A background (Fermi edge and spline) has been subtracted to obtain panel (c).

The valence band spectral density of GNRs obtained following this second route is reported in Fig. S4. The delocalized charge density in both the bisanthene units and GNRs leads to a spectral density broadened with respect to the better defined peaks for DDBA molecules and polyanthryl deposited at RT. This charge delocalization is also reflected in the broader absorption at the C-K edge,[S1] suggesting a redistribution of the LUMO states, as shown in the theoretical predictions. The coexistence of bisanthene units and GNR strands of different lengths, lying flat in the Au reconstructed channels, leads to a superimposition of different contributions to the spectral density. The presence of different species on the 1×4 reconstructed channels and the presence of other Au reconstructions[S1] strongly influence the distribution of the spectral density, as clearly described by the comparison of the theoretical DOS with different GNR-substrate configurations (see main paper). Eventually, this hinders the detection of the electronic state dispersion along the GNR direction.

# References


(S1) Massimi, L.; Ourdjini, O.; Lafferentz, L.; Koch, M.; Grill, L.; Cavaliere, E.; Gavioli, L.; Cardoso, C.; Prezzi, D.; Molinari, E. et al. Surface-Assisted Reactions toward Formation of Graphene Nanoribbons on Au(110) Surface. *J. Phys. Chem. C* **2015**, *119*, 2427–2437.

(S2) Simonov, K. A.; Vinogradov, N. A.; Vinogradov, A. S.; Generalov, A. V.; Zagrebina, E. M.; Svirskiy, G. I.; Cafolla, A. A.; Carpy, T.; Cunniffe, J. P.; Taketsugu, T. et al. From Graphene Nanoribbons on Cu(111) to Nanographene on Cu(110): Critical Role of Substrate Structure in the Bottom-up Fabrication Strategy. *ACS Nano* **2015**, *9*, 8997–9011.
